# Supplementary material for: Unsupervised Out-of-Domain Detection via Pre-trained Transformers
Source: arXiv:2106.00948 source file (2022-05-20)
Supplement: Supplementary file 1 [file appendix.tex]

\newpage

\begin{center}
\Large
\textbf{Appendix}
\end{center}

\section{Examples of CLINIC150 Dataset}
Table~\ref{tab:example_sentences} provides some examples of both in-domain and out-domain data in the CLINIC150. 
The intent labels are manually labeled, but are not used in our experiments. 
\begin{table*}[h]
    \centering
    \setlength{\tabcolsep}{6pt}
    
    \begin{tabular}{ l l l }
    \toprule
    \textbf{Type~~~~~~~~~} & \textbf{Intent~~~~~~~~~~~~~~~~~~~~~~} & \textbf{Sentence}~~~~~~~~~~~~~~~~~~~~~~\\
        \hline
      In-Domain & Transfer & \emph{move 100 dollars from my savings to my checking}\\
      In-Domain & PTO Request & \emph{let me know how to make a vacation request}\\
      In-Domain & Change Language & \textit{switch the language setting over to german}\\
      In-Domain & Distance & \emph{tell the miles it will take to get to las vegas from san diego}\\
      In-Domain & Travel Suggestion & \emph{what sites are there to see when in evans}\\
      In-Domain & Todo List Update & \textit{nuke all items on my todo list}\\
      In-Domain & Text & \emph{send a text to mom saying i'm on my way}\\
      In-Domain & Food Last & \emph{is rice ok after 3 days in the refrigerator}\\
      In-Domain & Tell Joke & \emph{can you tell me a joke about politicians}\\
      In-Domain & Rewards Balance & \emph{how high are the rewards on my discover card}\\
    \hline
  Out-of-Domain & - &\textit{how are my sports teams doing}\\
  Out-of-Domain & - & \textit{create a contact labeled mom}\\
  Out-of-Domain & - & \textit{what's the extended zipcode for my address}\\
    \bottomrule
\end{tabular}
\caption{Examples of CLINIC150.}
\label{tab:example_sentences}
\end{table*}
\newpage

\section{Additional Experimental Results}
\label{sec:appendix}
Table~\ref{tab:results-cls} and Table~\ref{tab:results-average} show the results of using [CLS] or averaging token embeddings at each layer of (Ro)BERT(a) models. We find that the best results of averaged embedding outperform that of using [CLS].
It is also interesting to see the best performance of [CLS] comes from the top layers, while averaged embedding benefits more from the bottom. 
When the representations of the top layer are used, the method based on [CLS] token is better than that based on taking the average. 

\begin{table*}[h]
\centering
\setlength{\tabcolsep}{3pt}
		
\scalebox{0.9}{
\begin{tabular}{lcccc|cccc}
\toprule
Layer & \multicolumn{4}{c}{BERT} & \multicolumn{4}{c}{RoBERTa} \\ \hline
           & AUROC & DTACC & AUIN  & AUOUT   & AUROC & DTACC & AUIN  & AUOUT\\ \hline
1 &    $\textbf{61.83}$ &  \textbf{59.31} & \textbf{87.63} &  24.17  & 53.36 & 53.32 & 83.07 & 20.60 \\
2 &    57.30 &  54.89 & 85.52 &  23.56  & 51.58  & 51.47 & 82.61 &  19.08 \\
3 &    56.63 &  55.68 & 84.42 &  22.47 & 53.76 & 53.73 & 84.81 & 18.94\\
4 &    56.76 &  55.37 & 84.97 &  22.12 & 58.25 & 56.05 & 86.19 & 22.88\\
5 &    61.55 &  58.62 & 86.83 &  \textbf{26.33} & \textbf{59.90} & \textbf{57.56} & \textbf{86.77} & \textbf{22.69} \\
6 &    58.76 &  57.76 & 84.87 &  24.21 & 57.53 & 56.28 & 85.57 & 21.33 \\
7 &    58.17 &  56.46 & 85.41 &  22.80 & 55.48 & 54.46 & 84.83 & 20.31 \\
8 &    56.34 & 55.07 & 84.16  & 23.45  & 56.21 & 55.41 & 84.87 & 20.83 \\
9 &    61.79 & 58.63 & 86.75 & 25.37 & 52.69 & 53.38 & 83.17 & 18.55 \\
10  &    52.88 & 53.87 & 84.55 & 18.44  & 50.95 & 52.91 & 83.48 & 17.67 \\
11  &  60.30 & 58.48 & 86.95 & 23.16 & 55.62 & 55.07 & 85.02 & 20.62   \\
12  & 60.24 & 58.51 & 86.11 & 23.97 & 55.63 & 54.64 & 84.61 & 21.24    \\
\bottomrule
\end{tabular}
}
\caption{Out-of-domain sample detection performance on the CLINIC150 dataset for each layer of BERT/RoBERTa. The embedding of \textbf{[CLS]} token represents the whole sequence. Layer 1 indicates the top layer and layer 12 is the bottom layer right after the word embedding layer. }
\label{tab:results-cls}
\end{table*}

\begin{table*}[h]
\centering
 \setlength{\tabcolsep}{3pt}
		
\scalebox{0.9}{
\begin{tabular}{lcccc|cccc}
\toprule
Layer & \multicolumn{4}{c}{BERT} & \multicolumn{4}{c}{RoBERTa} \\ \hline
           & AUROC & DTACC & AUIN  & AUOUT   & AUROC & DTACC & AUIN  & AUOUT\\ \hline
1 & 60.21 & 57.96 & 85.92 & 24.85 & 51.58 & 51.47 & 82.61 & 19.08 \\
2 & 58.97 & 57.38 & 86.39 & 23.15 & 55.50 & 55.08 & 85.06 & 19.51 \\
3 & 55.41 & 55.01 & 84.87 & 20.69 & 56.22 & 55.41 & 85.32 & 19.98 \\
4 & 56.47 & 54.93 & 85.41 & 21.44 & 56.45 & 55.53 & 85.44 & 20.08 \\
5 & 56.73 & 55.16 & 85.73 & 21.53 & 55.95 & 55.44 & 85.20 & 19.83 \\
6 & 63.02 & 60.12 & 87.62 & 26.18 & 56.37 & 55.53 & 85.35 & 20.06 \\
7 & 61.04 & 58.88 & 87.17 & 23.42 & 56.64 & 55.52 & 85.37 & 20.33 \\
8 & 61.85 & 59.19 & 86.63 & 25.27 & 57.07 & 55.92 & 85.52 & 20.58 \\
9 & 60.94 & 58.69 & 86.81 & 23.30 & 57.80 & 56.48 & 85.83 & 20.94 \\
10 & 59.20 & 57.02 & 86.50 & 22.16 & 58.46 & \textbf{57.37} & 86.07 & 21.32 \\
11 & 58.57 & 56.40 & 86.65 & 22.29 & \textbf{58.89} & 57.23 & 86.16 & \textbf{21.78} \\
12 & \textbf{64.61} & \textbf{60.97} & \textbf{88.44} & \textbf{26.71} & 58.49 & 57.24 & \textbf{86.48} & 20.99 \\
\bottomrule
\end{tabular}
}
\caption{Out-of-domain sample detection performance on the CLINIC150 dataset for each layer of BERT/RoBERTa. The \textbf{average} of all contexualized embeddings in the same layer represents the sequence input. Layer 1 indicates the top layer and layer 12 is the bottom layer right after the embedding layer.}
\label{tab:results-average}
\end{table*}
